# Supplementary material for: Everything at Once -- Multi-modal Fusion Transformer for Video Retrieval
Source: arXiv:2112.04446 source file (2022-08-18)
Supplement: Supplementary file 1 [file retrieval.tex]

\begin{table*}
    % \tablestyle{3pt}{1.05}
    \centering
    % \resizebox{1\linewidth}{!}{
    \begin{tabular}{@{}l|c|c|cccc|cccc@{}}
    	\toprule

        Visual & Training & Retrieval & \multicolumn{4}{c}{YouCook2} & \multicolumn{4}{c}{MSR-VTT} \\ 
    	   Backbone & Modalities & & R@1$\uparrow$  & R@5$\uparrow$ & R@10$\uparrow$ & MedR$\downarrow$ & R@1$\uparrow$ & R@5$\uparrow$  & R@10$\uparrow$ & MedR$\downarrow$\\ 
    	\midrule
    	R152 + RX101 & $tva$ & $t \to v$ & 10.7 & 27.9 & 38.9 & 19 & 10.3 & 24.6 & 35.3 & 25\\
    	S3D$\dagger$ & $tva$ & $t \to v$ & 19.8 & 42.9 & 55.1 & 8 & 9.9 & 24.0 & 32.6 & 28 \\
    	CLIP$\ddagger$ & $tva$ & $t \to v$ & 12.2 & 29.7 & 40.2 & 18 & 14.6 & 33.8 & 43.4 & 14 \\
    	S3D$\dagger$ + CLIP$\ddagger$ & $tva$ & $t \to v$ & 20.4 & 44.4 & 57.2 & 7 & 14.4 & 33.6 & 44.8 & 13 \\
    	\midrule
    	R152 + RX101 & $tva$ & $t \to va$ & 20.0 & 40.7 & 51.3 & 10 & 8.9 & 23.8 & 31.8 & 30  \\
    	S3D$\dagger$ & $tva$ & $t \to va$ & 24.6 & 48.3 & 60.4 & 6 & 9.3 & 22.9 & 31.2 & 35 \\
    	CLIP$\ddagger$ & $tva$ & $t \to va$ & 20.3 & 42.7 & 54.0 & 8 & 12.6 & 29.0 & 38.7 & 18 \\
    	S3D$\dagger$ + CLIP$\ddagger$ & $tva$ & $t \to va$ & 26.2 & 49.6 & 60.8 & 6 & 13.4 & 28.8 & 37.7 & 19 \\

    \bottomrule
    \end{tabular}
    \caption{\todo{}
    \label{tab:sup_retrieval}
    }
    % \vspace{-0.3cm}
    % \vspace{-0.25cm}
\end{table*}
